# Supplementary material for: Dynamic Bounds on Stochastic Chemical Kinetic Systems Using Semidefinite Programming
Source: arXiv:1802.04409 source file (2018-03-09)
Supplement: Supplementary file 1 [file Supplementary_Material.pdf]

# Supplementary Material

Garrett R. Dowdy and Paul I. Barton

March 6, 2018

# 1 Introduction

This document is intended to accompany the paper entitled "Dynamic Bounds on Stochastic Chemical Kinetic Systems Using Semidefinite Programming" by Garrett R. Dowdy and Paul I. Barton.

# 2 Complex Eigenvalues

In Section VI, we stated that it was possible to derive augmented forms of the bounding SDPs appearing in our paper that account for the imaginary components of eigenvalues. In this section, we explain how those augmented SDPs are constructed.

## 2.1 Linear Equations

Previously, we derived the equation

$$\boldsymbol{\mu}_L(T) - e^{\rho T}\boldsymbol{\mu}_L(0) = (\mathbf{A}_L - \rho\mathbf{I})\int_0^T e^{\rho(T-t)}\boldsymbol{\mu}_L(t)dt + \mathbf{A}_H\int_0^T e^{\rho(T-t)}\boldsymbol{\mu}_H(t)dt. \tag{1}$$

While we derived this equation assuming that $\rho \in \mathbb{R}$, it is equally valid for any $\rho \in \mathbb{C}$, where $\mathbb{C}$ is the set of complex numbers. Substituting $\rho = a + bi$ into the equation, we obtain

$$\begin{aligned}\boldsymbol{\mu}_L(T) - e^{(a+bi)T}\boldsymbol{\mu}_L(0) &= (\mathbf{A}_L - (a+bi)\mathbf{I})\int_0^T e^{(a+bi)(T-t)}\boldsymbol{\mu}_L(t)dt + \mathbf{A}_H\int_0^T e^{(a+bi)(T-t)}\boldsymbol{\mu}_H(t)dt \\ \boldsymbol{\mu}_L(T) - e^{aT}e^{biT}\boldsymbol{\mu}_L(0) &= (\mathbf{A}_L - (a+bi)\mathbf{I})\int_0^T e^{a(T-t)}e^{bi(T-t)}\boldsymbol{\mu}_L(t)dt + \mathbf{A}_H\int_0^T e^{a(T-t)}e^{bi(T-t)}\boldsymbol{\mu}_H(t)dt.\end{aligned} \tag{2}$$

Using Euler's formula, this becomes

$$\begin{aligned}\boldsymbol{\mu}_L(T) - &e^{aT}(\cos(bT) + i\sin(bT))\boldsymbol{\mu}_L(0) \\ &= (\mathbf{A}_L - (a+bi)\mathbf{I})\int_0^T e^{a(T-t)}(\cos(b(T-t)) + i\sin(b(T-t)))\boldsymbol{\mu}_L(t)dt \\ &\quad + \mathbf{A}_H\int_0^T e^{a(T-t)}(\cos(b(T-t)) + i\sin(b(T-t)))\boldsymbol{\mu}_H(t)dt\end{aligned} \tag{3}$$

Next, through simple but tedious algebraic manipulations, each side of this equation can then be separated into the real and imaginary parts:

$$\begin{aligned}(\boldsymbol{\mu}_L(T) - e^{aT}\cos(bT)\boldsymbol{\mu}_L(0)) - ie^{aT}\sin(bT)\boldsymbol{\mu}_L(0) \\ = (\mathbf{A}_L - a\mathbf{I})\int_0^T e^{a(T-t)}\cos(b(T-t))\boldsymbol{\mu}_L(t)dt + b\int_0^T e^{a(T-t)}\sin(b(T-t))\boldsymbol{\mu}_L(t)dt \\ + \mathbf{A}_H\int_0^T e^{a(T-t)}\cos(b(T-t))\boldsymbol{\mu}_H(t)dt \\ + i(\mathbf{A}_L - a\mathbf{I})\int_0^T e^{a(T-t)}\sin(b(T-t))\boldsymbol{\mu}_L(t)dt - ib\int_0^T e^{a(T-t)}\cos(b(T-t))\boldsymbol{\mu}_L(t)dt \\ + i\mathbf{A}_H\int_0^T e^{a(T-t)}\sin(b(T-t))\boldsymbol{\mu}_H(t)dt\end{aligned} \tag{4}$$

This equation holds if and only if the real part of the left-hand side equals the real part of the right-hand side, and the imaginary part of the left-hand side equals the imaginary part of the right-hand side. So, it is equivalent to the following two equations:

$$\begin{aligned}\boldsymbol{\mu}_L(T) - e^{aT}\cos(bT)\boldsymbol{\mu}_L(0) \\ = (\mathbf{A}_L - a\mathbf{I})\int_0^T e^{a(T-t)}\cos(b(T-t))\boldsymbol{\mu}_L(t)dt + b\int_0^T e^{a(T-t)}\sin(b(T-t))\boldsymbol{\mu}_L(t)dt \\ + \mathbf{A}_H\int_0^T e^{a(T-t)}\cos(b(T-t))\boldsymbol{\mu}_H(t)dt\end{aligned} \tag{5}$$

$$\begin{aligned}-e^{aT}\sin(bT)\boldsymbol{\mu}_L(0) \\ = (\mathbf{A}_L - a\mathbf{I})\int_0^T e^{a(T-t)}\sin(b(T-t))\boldsymbol{\mu}_L(t)dt - b\int_0^T e^{a(T-t)}\cos(b(T-t))\boldsymbol{\mu}_L(t)dt \\ + \mathbf{A}_H\int_0^T e^{a(T-t)}\sin(b(T-t))\boldsymbol{\mu}_H(t)dt\end{aligned} \tag{6}$$

Now, just as we defined the variables $\mathbf{z}_L^{(\rho)}$ and $\mathbf{z}_H^{(\rho)}$ as a shorthand representation of the integrals appearing in (1), we will similarly define shorthand names for the integrals appearing in (5) and (6). In particular, defining

$$\begin{aligned}z_{\mathbf{j}}^{(a\cos b)} &\equiv \int_0^T e^{a(T-t)}\cos(b(T-t))\mu_{\mathbf{j}}(t)dt, \quad \forall \mathbf{j} \in \mathbb{N}^{\hat{N}}, \\ z_{\mathbf{j}}^{(a\sin b)} &\equiv \int_0^T e^{a(T-t)}\sin(b(T-t))\mu_{\mathbf{j}}(t)dt, \quad \forall \mathbf{j} \in \mathbb{N}^{\hat{N}},\end{aligned} \tag{7}$$

we can write the Equations (5) and (6) more concisely as

$$\boldsymbol{\mu}_L(T) - e^{aT}\cos(bT)\boldsymbol{\mu}_L(0) = (\mathbf{A}_L - a\mathbf{I})\mathbf{z}_L^{(a\cos b)} + b\mathbf{z}_L^{(a\sin b)} + \mathbf{A}_H\mathbf{z}_H^{(a\cos b)} \tag{8}$$

$$-e^{aT}\sin(bT)\boldsymbol{\mu}_L(0) = (\mathbf{A}_L - a\mathbf{I})\mathbf{z}_L^{(a\sin b)} - b\mathbf{z}_L^{(a\cos b)} + \mathbf{A}_H\mathbf{z}_H^{(a\sin b)} \tag{9}$$

Now for a sanity check. Since the above equations equations were derived assuming any values $a, b \in \mathbb{R}$, they should also hold in the special case when $b = 0$. In this case, $\rho = a + bi = a$ is just a real number, and we would expect Equations (8) and (9) to reduce to Equation (1), which we derived assuming that $\rho$ was real. Indeed, this is true. Using the definitions given in Equation (7), we see that Equations (8) reduces

to Equation (1) and (9) reduces to the vacuously true statement $0 = 0$. This result shows that Equations (8) and (9) are a consistent generalization of our previous work.

Of course, to use these necessary conditions as constraints in an optimization problem, we need to state them in terms of the appropriate decision variable proxies:

$$\tilde{\boldsymbol{\mu}}_L(T) - e^{aT}\cos(bT)\boldsymbol{\mu}_L(0) = (\mathbf{A}_L - a\mathbf{I})\tilde{\mathbf{z}}_L^{(a\cos b)} + b\tilde{\mathbf{z}}_L^{(a\sin b)} + \mathbf{A}_H\tilde{\mathbf{z}}_H^{(a\cos b)} \tag{10}$$

$$-e^{aT}\sin(bT)\boldsymbol{\mu}_L(0) = (\mathbf{A}_L - a\mathbf{I})\tilde{\mathbf{z}}_L^{(a\sin b)} - b\tilde{\mathbf{z}}_L^{(a\cos b)} + \mathbf{A}_H\tilde{\mathbf{z}}_H^{(a\sin b)} \tag{11}$$

## 2.2 Linear Matrix Inequalities and Second-Order Cone Constraints

As was the case with Equation (1), Equations (10) and (11) are of limited value unless we further constrain the values of $\tilde{z}_{\mathbf{j}}^{(a\cos b)}$ and $\tilde{z}_{\mathbf{j}}^{(a\cos b)}$. These additional constraints will take the form of LMIs and second-order cone constraints.

First, by the trigonometric identity, we have

$$\sin^2(b(T-t)) + \cos^2(b(T-t)) = 1, \quad \forall t \in [0,T]. \tag{12}$$

It follows trivially, that

$$\sin^2(b(T-t)) + \cos^2(b(T-t)) \leq 1, \quad \forall t \in [0,T]. \tag{13}$$

Now, pick an arbitrary $\mathbf{j} \in \mathbb{N}^{\hat{N}}$. Multiplying both sides of the above inequality by $\mu_{\mathbf{j}}^2(t)$ gives

$$\mu_{\mathbf{j}}^2(t)\sin^2(b(T-t)) + \mu_{\mathbf{j}}^2(t)\cos^2(b(T-t)) \leq \mu_{\mathbf{j}}^2(t), \quad \forall t \in [0,T]. \tag{14}$$

Taking the square root of both sides gives

$$\sqrt{\mu_{\mathbf{j}}^2(t)\sin^2(b(T-t)) + \mu_{\mathbf{j}}^2(t)\cos^2(b(T-t))} = \left\| \begin{bmatrix} \mu_{\mathbf{j}}(t)\sin(b(T-t)) \\ \mu_{\mathbf{j}}(t)\cos(b(T-t)) \end{bmatrix} \right\|_2 \leq |\mu_{\mathbf{j}}(t)| = \mu_{\mathbf{j}}(t), \quad \forall t \in [0,T]. \tag{15}$$

The last equality assumes that $\mu_{\mathbf{j}}(t) \geq 0$. This will be true as long as we choose the appropriate representation of our state space. It is true, in particular, for our chosen representation in terms of independent species.

Multiplying both sides of the above inequality by $e^{a(T-t)}$ and integrating from $t = 0$ to $t = T$ gives

$$\int_0^T e^{a(T-t)} \left\| \begin{bmatrix} \mu_{\mathbf{j}}(t)\sin(b(T-t)) \\ \mu_{\mathbf{j}}(t)\cos(b(T-t)) \end{bmatrix} \right\|_2 dt \leq \int_0^T e^{a(T-t)}\mu_{\mathbf{j}}(t)dt = z_{\mathbf{j}}^{(a)} \tag{16}$$

Focusing on the left-hand side, we can use Jensen's Inequality to obtain

$$\begin{aligned} \int_0^T e^{a(T-t)} \left\| \begin{bmatrix} \mu_{\mathbf{j}}(t)\sin(b(T-t)) \\ \mu_{\mathbf{j}}(t)\cos(b(T-t)) \end{bmatrix} \right\|_2 dt &= \int_0^T \left\| \begin{bmatrix} e^{a(T-t)}\mu_{\mathbf{j}}(t)\sin(b(T-t)) \\ e^{a(T-t)}\mu_{\mathbf{j}}(t)\cos(b(T-t)) \end{bmatrix} \right\|_2 dt \\ &\geq \left\| \int_0^T \begin{bmatrix} e^{a(T-t)}\mu_{\mathbf{j}}(t)\sin(b(T-t)) \\ e^{a(T-t)}\mu_{\mathbf{j}}(t)\cos(b(T-t)) \end{bmatrix} dt \right\|_2 \\ &= \left\| \begin{bmatrix} \int_0^T e^{a(T-t)}\mu_{\mathbf{j}}(t)\sin(b(T-t))dt \\ \int_0^T e^{a(T-t)}\mu_{\mathbf{j}}(t)\cos(b(T-t))dt \end{bmatrix} \right\|_2 \\ &= \left\| \begin{bmatrix} z_{\mathbf{j}}^{(a\sin b)} \\ z_{\mathbf{j}}^{(a\cos b)} \end{bmatrix} \right\|_2 \end{aligned} \tag{17}$$

Combining this result with Inequality (16), we have the following second-order cone constraint involving the quantities $z_{\mathbf{j}}^{(a\sin b)}$, $z_{\mathbf{j}}^{(a\cos b)}$, and $z_{\mathbf{j}}^{(a)}$.

$$\left\| \begin{bmatrix} z_{\mathbf{j}}^{(a\sin b)} \\ z_{\mathbf{j}}^{(a\cos b)} \end{bmatrix} \right\|_2 \leq z_{\mathbf{j}}^{(a)}, \tag{18}$$

which, of course, can also be written for our proxy variables $\tilde{z}_{\mathbf{j}}^{(a\sin b)}$, $\tilde{z}_{\mathbf{j}}^{(a\cos b)}$, and $\tilde{z}_{\mathbf{j}}^{(a)}$.

Now, unless we constrain the value of $\tilde{z}_{\mathbf{j}}^{(a)}$, this inequality is of no use to us; if $\tilde{z}_{\mathbf{j}}^{(a)}$ can be made arbitrarily large, then $\tilde{z}_{\mathbf{j}}^{(a\sin b)}$ and $\tilde{z}_{\mathbf{j}}^{(a\cos b)}$ can take any value. Fortunately, we already know exactly how to constrain $\tilde{z}_{\mathbf{j}}^{(a)}$. It is subject to exactly the same constraints that we derived earlier for $\tilde{z}_{\mathbf{j}}^{(\rho)}$, when we were considering exclusively real values of $\rho$. First, we have the linear equalities,

$$\tilde{\boldsymbol{\mu}}_L(T) - e^{aT}\boldsymbol{\mu}_L(0) = (\mathbf{A}_L - a\mathbf{I})\tilde{\mathbf{z}}_L^{(a)} + \mathbf{A}_H\tilde{\mathbf{z}}_H^{(a)}. \tag{19}$$

Second, we have the LMIs implied by membership in the cone $C_n(\boldsymbol{\alpha}, \boldsymbol{\beta})$,

$$\tilde{\mathbf{z}}^{(a)} \in C_n(\boldsymbol{\alpha}, \boldsymbol{\beta}) \tag{20}$$

## 2.3 Bringing It All Together

To summarize, if you wish to use a complex $\rho = a + bi$ in the bound calculation, we need to include the following constraints in the optimization problem:

$$\tilde{\boldsymbol{\mu}}_L(T) - e^{aT}\cos(bT)\boldsymbol{\mu}_L(0) = (\mathbf{A}_L - a\mathbf{I})\tilde{\mathbf{z}}_L^{(a\cos b)} + b\tilde{\mathbf{z}}_L^{(a\sin b)} + \mathbf{A}_H\tilde{\mathbf{z}}_H^{(a\cos b)} \tag{21}$$

$$-e^{aT}\sin(bT)\boldsymbol{\mu}_L(0) = (\mathbf{A}_L - a\mathbf{I})\tilde{\mathbf{z}}_L^{(a\sin b)} - b\tilde{\mathbf{z}}_L^{(a\cos b)} + \mathbf{A}_H\tilde{\mathbf{z}}_H^{(a\sin b)} \tag{22}$$

$$\left\| \begin{bmatrix} \tilde{z}_{\mathbf{j}}^{(a\sin b)} \\ \tilde{z}_{\mathbf{j}}^{(a\cos b)} \end{bmatrix} \right\|_2 \leq \tilde{z}_{\mathbf{j}}^{(a)}, \quad \forall \mathbf{j} \in \mathbb{N}^{\hat{N}} \text{s.t. } |\mathbf{j}| \leq M \tag{23}$$

$$\tilde{\boldsymbol{\mu}}_L(T) - e^{aT}\boldsymbol{\mu}_L(0) = (\mathbf{A}_L - \rho\mathbf{I})\tilde{\mathbf{z}}_L^{(a)} + \mathbf{A}_H\tilde{\mathbf{z}}_H^{(a)} \tag{24}$$

$$\tilde{\mathbf{z}}^{(a)} \in C_n(\boldsymbol{\alpha}, \boldsymbol{\beta}) \tag{25}$$

As a reminder, the $M$ appearing in Constraint (23) is the order of the highest-order moment appearing in $\tilde{\mathbf{z}}_H^{(a)}$ (and $\boldsymbol{\mu}_H$).

## 2.4 Complex Conjugates

Now, recall that the values of $\rho$ that we use are intended to estimate eigenvalues of the infinitesimal generator matrix $\mathbf{G}$. All of the elements of this matrix are real. This implies that any complex eigenvalues occur in conjugate pairs. Thus, if we are using $\rho = a + bi$ as an estimate of one of the eigenvalues, it seems that we should be using $\rho = a - bi$ also. However, one can show that if we write out Conditions (21) - (25) for $\rho = a + bi$, it is redundant to also write out these conditions for $\rho = a - bi$.

To see this, suppose we write out

$$\tilde{\boldsymbol{\mu}}_L(T) - e^{aT}\cos(bT)\boldsymbol{\mu}_L(0) = (\mathbf{A}_L - a\mathbf{I})\tilde{\mathbf{z}}_L^{(a\cos -b)} - b\tilde{\mathbf{z}}_L^{(a\sin -b)} + \mathbf{A}_H\tilde{\mathbf{z}}_H^{(a\cos -b)}, \tag{26}$$

$$e^{aT}\sin(bT)\boldsymbol{\mu}_L(0) = (\mathbf{A}_L - a\mathbf{I})\tilde{\mathbf{z}}_L^{(a\sin -b)} + b\tilde{\mathbf{z}}_L^{(a\cos -b)} + \mathbf{A}_H\tilde{\mathbf{z}}_H^{(a\sin -b)}, \tag{27}$$

$$\left\|\left[\begin{array}{c}\tilde{z}_{\mathbf{j}}^{(a\sin -b)}\\ \tilde{z}_{\mathbf{j}}^{(a\cos -b)}\end{array}\right]\right\|_2 \leq \tilde{z}_{\mathbf{j}}^{(a)}, \quad \forall \mathbf{j}\in\mathbb{N}^{\hat{N}} \text{s.t. } |\mathbf{j}|\leq M. \tag{28}$$

to supplement Conditions (21) - (25) as constraints in our optimization problem. (Conditions (24)- (25) are not copied, as they have no dependence on the sign of $b$, and are thus obviously redundant.) The question is: does the addition of Constraints (26) - (28) further constrain the set of feasible vectors $\tilde{\boldsymbol{\mu}}_L(T)$? The answer is "no", because if we have vectors $\tilde{\boldsymbol{\mu}}_L(T)$, $\tilde{\mathbf{z}}^{(a\cos b)}$, $\tilde{\mathbf{z}}^{(a\sin b)}$, and $\tilde{\mathbf{z}}^{(a)}$ which satisfy Constraints (21) - (25), we can trivially construct vectors $\tilde{\mathbf{z}}^{(a\cos -b)}$ and $\tilde{\mathbf{z}}^{(a\sin -b)}$ which satisfy Constraints (26) - (28). We simply set $\tilde{\mathbf{z}}^{(a\cos -b)} \equiv \tilde{\mathbf{z}}^{(a\cos b)}$ and $\tilde{\mathbf{z}}^{(a\sin -b)} \equiv -\tilde{\mathbf{z}}^{(a\sin b)}$. This means that the addition of Constraints (26) - (28) has no effect on the set of feasible vectors $\tilde{\boldsymbol{\mu}}_L(T)$. In other words, Constraints (26) - (28) are redundant.

From another perspective, this conclusion is not surprising. If we start with Conditions (21) - (25), written for the true quantities $\boldsymbol{\mu}_L(T)$, $\mathbf{z}^{(a\cos b)}$, $\mathbf{z}^{(a\sin b)}$, and $\mathbf{z}^{(a)}$, and we expand the definitions of $\mathbf{z}^{(a\cos b)}$ and $\mathbf{z}^{(a\sin b)}$ into integral form, we see that replacing $b$ with $-b$ yields an exactly equivalent set of conditions.

To summarize, if we write Conditions (21) - (25) for $\rho = a + bi$, we don't need to worry about also writing them for $\rho = a - bi$ as the second set of conditions is implied by the first.

## 2.5 An Augmented SDP

So suppose we wanted to construct an SDP for bounding a stochastic chemical kinetic system using a set $\mathcal{R}$ containing both real and complex values of $\rho$. What does this look like?

Suppose that there are $|\mathcal{R}|$ values of $\rho$, which can be written as $\mathcal{R} \equiv \{\rho_1, \ldots, \rho_{|\mathcal{R}|}\} \equiv \{a_1 + b_1 i, \ldots, a_{|\mathcal{R}|} + b_{|\mathcal{R}|} i\}$. For the reasons discussed in the previous section we do not want this set to contain any complex conjugate pairs. Let $J \equiv \{1, \ldots, |\mathcal{R}|\}$ and let $J_{\mathbb{C}} \equiv \{j \in J : b_j \neq 0\}$. In other words, $J_{\mathbb{C}}$ is the set of indices corresponding to the complex values of $\rho_j$.

Then, we can write the SDP for calculating an upper bound on the mean molecular count of species $i$ as follows:

$$\begin{aligned}
\max_{\substack{\tilde{\boldsymbol{\mu}}(T),\\ \tilde{\mathbf{z}}^{(a_j)},\forall j\in J,\\ \tilde{\mathbf{z}}^{(a_j\cos b_j)},\forall j\in J_{\mathbb{C}},\\ \tilde{\mathbf{z}}^{(a_j\sin b_j)},\forall j\in J_{\mathbb{C}}}} \quad & \tilde{\mu}_{\mathbf{e}_i}(T)\\
\text{s.t.} \quad & \tilde{\mu}_{\mathbf{0}}(T) = 1,\\
& \tilde{\boldsymbol{\mu}}(T) \in C_n(\boldsymbol{\alpha},\boldsymbol{\beta}),\\
& \tilde{\mathbf{z}}^{(a_j)} \in C_n(\boldsymbol{\alpha},\boldsymbol{\beta}), \quad \forall j \in J,\\
& \tilde{\boldsymbol{\mu}}_L(T) - e^{a_jT}\boldsymbol{\mu}_L(0) = (\mathbf{A}_L - a_j\mathbf{I})\tilde{\mathbf{z}}_L^{(a_j)} + \mathbf{A}_H\tilde{\mathbf{z}}_H^{(a_j)}, \quad \forall j\in J,\\
& \tilde{\boldsymbol{\mu}}_L(T) - e^{a_jT}\cos(b_jT)\boldsymbol{\mu}_L(0) = (\mathbf{A}_L - a_j\mathbf{I})\tilde{\mathbf{z}}_L^{(a_j\cos b_j)} + b_j\tilde{\mathbf{z}}_L^{(a_j\sin b_j)} + \mathbf{A}_H\tilde{\mathbf{z}}_H^{(a_j\cos b_j)}, \quad \forall j\in J_{\mathbb{C}},\\
& -e^{a_jT}\sin(b_jT)\boldsymbol{\mu}_L(0) = (\mathbf{A}_L - a_j\mathbf{I})\tilde{\mathbf{z}}_L^{(a_j\sin b_j)} - b_j\tilde{\mathbf{z}}_L^{(a_j\cos b_j)} + \mathbf{A}_H\tilde{\mathbf{z}}_H^{(a_j\sin b_j)}, \quad \forall j\in J_{\mathbb{C}},\\
& \left\|\left[\begin{array}{c}\tilde{z}_{\mathbf{j}}^{(a_j\sin b_j)}\\ \tilde{z}_{\mathbf{j}}^{(a_j\cos b_j)}\end{array}\right]\right\|_2 \leq \tilde{z}_{\mathbf{j}}^{(a_j)}, \quad \forall \mathbf{j}\in\mathbb{N}^{\hat{N}}\text{s.t. } |\mathbf{j}|\leq M, \quad \forall j\in J_{\mathbb{C}}.
\end{aligned} \tag{29}$$

Technically, this is not an SDP, because of the presence of the second order cone constraints. However, each of these second order cone constraints can be written equivalently as an LMI, so this technicality is of no consequence.

# 3 The Absence of the Closure Problem

In Section VII of our paper, we observed that when our bounding method is applied to systems which do not exhibit the closure problem, the bounds are often perfect. In this section, we give some insight into why this is the case.

## 3.1 Theoretical Reasoning

When a system does not suffer from the closure problem, the $\mathbf{A}_H$ matrix appearing in Equation (1) is all zeros. This means that the associated constraint simplifies to

$$\tilde{\boldsymbol{\mu}}_L(T) - e^{\rho T}\boldsymbol{\mu}_L(0) = (\mathbf{A}_L - \rho\mathbf{I})\tilde{\mathbf{z}}_L^{(\rho)}. \tag{30}$$

Now, to simplify the discussion, let us assume that the matrix has $\mathbf{A}_L \in \mathbb{R}^{d\times d}$ has $d$ distinct eigenvalues $\{\lambda_1, \dots, \lambda_d\}$. It follows that $\mathbf{A}_L$ is has $d$ linearly independent eigenvectors $\{\mathbf{v}_1, \dots, \mathbf{v}_d\} \subset \mathbb{C}^d$. Furthermore, if we let $\mathbf{V} \equiv [\mathbf{v}_1 \dots \mathbf{v}_d]$, then

$$\mathbf{A}_L = \mathbf{V}\boldsymbol{\Lambda}\mathbf{V}^{-1}, \tag{31}$$

where $\boldsymbol{\Lambda} \equiv \mathrm{diag}(\lambda_1, \dots, \lambda_d)$. It follows that

$$\mathbf{A}_L - \rho\mathbf{I} = \mathbf{V}\boldsymbol{\Lambda}\mathbf{V}^{-1} - \rho\mathbf{V}\mathbf{V}^{-1} = \mathbf{V}(\boldsymbol{\Lambda} - \rho\mathbf{I})\mathbf{V}^{-1}. \tag{32}$$

Then, Equation (30) becomes

$$\tilde{\boldsymbol{\mu}}_L(T) - e^{\rho T}\boldsymbol{\mu}_L(0) = \mathbf{V}(\boldsymbol{\Lambda} - \rho\mathbf{I})\mathbf{V}^{-1}\tilde{\mathbf{z}}_L^{(\rho)}. \tag{33}$$

Rearranging gives

$$\tilde{\boldsymbol{\mu}}_L(T) = \mathbf{V}(\boldsymbol{\Lambda} - \rho\mathbf{I})\mathbf{V}^{-1}\tilde{\mathbf{z}}_L^{(\rho)} + e^{\rho T}\boldsymbol{\mu}_L(0). \tag{34}$$

Now, suppose that we choose our values of $\rho$ to be $\mathcal{R} = \{\lambda_1, \dots, \lambda_d\}$. Then, enforcing Equation (34) for each $\rho \in \mathcal{R}$, we have

$$\begin{aligned}
\tilde{\boldsymbol{\mu}}_L(T) &= \mathbf{V}(\boldsymbol{\Lambda} - \lambda_1\mathbf{I})\mathbf{V}^{-1}\tilde{\mathbf{z}}_L^{(\lambda_1)} + e^{\lambda_1 T}\boldsymbol{\mu}_L(0),\\
\tilde{\boldsymbol{\mu}}_L(T) &= \mathbf{V}(\boldsymbol{\Lambda} - \lambda_2\mathbf{I})\mathbf{V}^{-1}\tilde{\mathbf{z}}_L^{(\lambda_2)} + e^{\lambda_2 T}\boldsymbol{\mu}_L(0),\\
&\vdots\\
\tilde{\boldsymbol{\mu}}_L(T) &= \mathbf{V}(\boldsymbol{\Lambda} - \lambda_d\mathbf{I})\mathbf{V}^{-1}\tilde{\mathbf{z}}_L^{(\lambda_d)} + e^{\lambda_d T}\boldsymbol{\mu}_L(0),
\end{aligned} \tag{35}$$

The first set of these equations specifies that $\tilde{\boldsymbol{\mu}}_L(T)$ is contained in an affine subspace spanned by the vectors $\{\mathbf{v}_2, \dots, \mathbf{v}_d\}$, with $\mathbf{v}_1$ omitted:

$$A_1 \equiv \left\{\mathbf{V}(\boldsymbol{\Lambda} - \lambda_1\mathbf{I})\mathbf{V}^{-1}\mathbf{z} + e^{\lambda_1 T}\boldsymbol{\mu}_L(0) : \mathbf{z} \in \mathbb{R}^d\right\}. \tag{36}$$

Similarly, the second set of equations specifies that $\tilde{\boldsymbol{\mu}}_L(T)$ is contained in an affine subspace spanned by the vectors $\{\mathbf{v}_1, \mathbf{v}_3 \dots, \mathbf{v}_d\}$, with $\mathbf{v}_2$ omitted:

$$A_2 \equiv \left\{\mathbf{V}(\boldsymbol{\Lambda} - \lambda_2\mathbf{I})\mathbf{V}^{-1}\mathbf{z} + e^{\lambda_2 T}\boldsymbol{\mu}_L(0) : \mathbf{z} \in \mathbb{R}^d\right\} \tag{37}$$

Continuing in this way, we see that $\tilde{\boldsymbol{\mu}}_L(T)$ is contained in all affine subspaces

$$A_j \equiv \left\{\mathbf{V}(\boldsymbol{\Lambda} - \lambda_j\mathbf{I})\mathbf{V}^{-1}\mathbf{z} + e^{\lambda_j T}\boldsymbol{\mu}_L(0) : \mathbf{z} \in \mathbb{R}^d\right\} \tag{38}$$

for $j \in \{1, \dots, d\}$. This implies that $\tilde{\boldsymbol{\mu}}_L(T)$ must lie in the intersection $\bigcap_{j\in\{1,\dots,d\}} A_j$. One can show that this intersection is nonempty and has exactly one point.

**Claim 1.** *The set* $\bigcap_{j\in\{1,\dots,d\}} A_j$ *is nonempty.*

*Proof.* The statement that $\bigcap_{j\in\{1,\dots,d\}} A_j$ is nonempty is equivalent to the statement that there exists some $(\tilde{\boldsymbol{\mu}}_L(T), \tilde{\mathbf{z}}_L^{(\lambda_1)}, \dots, \tilde{\mathbf{z}}_L^{(\lambda_d)}) \in \mathbb{R}^{d+d^2}$ satisfying Equation (35). This equation can be written equivalently in matrix-vector form:

$$\begin{bmatrix} \mathbf{I} & -\mathbf{V}(\boldsymbol{\Lambda}-\lambda_1\mathbf{I})\mathbf{V}^{-1} & \mathbf{0} & \dots & \mathbf{0} \\ \mathbf{I} & \mathbf{0} & -\mathbf{V}(\boldsymbol{\Lambda}-\lambda_2\mathbf{I})\mathbf{V}^{-1} & \dots & \mathbf{0} \\ \vdots & \vdots & \vdots & \ddots & \vdots \\ \mathbf{I} & \mathbf{0} & \mathbf{0} & \dots & -\mathbf{V}(\boldsymbol{\Lambda}-\lambda_d\mathbf{I})\mathbf{V}^{-1} \end{bmatrix} \begin{bmatrix} \tilde{\boldsymbol{\mu}}_L(T) \\ \tilde{\mathbf{z}}_L^{(\lambda_1)} \\ \tilde{\mathbf{z}}_L^{(\lambda_2)} \\ \vdots \\ \tilde{\mathbf{z}}_L^{(\lambda_d)} \end{bmatrix} = \begin{bmatrix} e^{\lambda_2 T}\boldsymbol{\mu}_L(0) \\ e^{\lambda_2 T}\boldsymbol{\mu}_L(0) \\ \vdots \\ e^{\lambda_d T}\boldsymbol{\mu}_L(0) \end{bmatrix} \tag{39}$$

This system of equations is guaranteed to have a solution if the leftmost matrix (call it $\mathbf{Q} \in \mathbb{R}^{d^2\times(d^2+d)}$) has $d^2$ linearly independent columns (i.e., if it's rank is $d^2$). To help us analyze its rank, we will pre-multiply by the invertible matrix

$$\begin{bmatrix} \mathbf{V}^{-1} & & \\ & \ddots & \\ & & \mathbf{V}^{-1} \end{bmatrix} \in \mathbb{R}^{d^2}, \tag{40}$$

and post-multiply by the invertible matrix

$$\begin{bmatrix} \mathbf{V} & & \\ & \ddots & \\ & & \mathbf{V} \end{bmatrix} \in \mathbb{R}^{d^2+d}. \tag{41}$$

The resulting matrix, which has the same rank as $\mathbf{Q}$, is

$$\begin{bmatrix} \mathbf{I} & -(\boldsymbol{\Lambda}-\lambda_1\mathbf{I}) & \mathbf{0} & \dots & \mathbf{0} \\ \mathbf{I} & \mathbf{0} & -(\boldsymbol{\Lambda}-\lambda_2\mathbf{I}) & \dots & \mathbf{0} \\ \vdots & \vdots & \vdots & \ddots & \vdots \\ \mathbf{I} & \mathbf{0} & \mathbf{0} & \dots & -(\boldsymbol{\Lambda}-\lambda_d\mathbf{I}) \end{bmatrix}. \tag{42}$$

From the sparsity pattern of this matrix, it follows that no row can be expressed as a linear combination of the others. It follows that each of the $d^2$ rows are linearly independent. This implies that the rank of $\mathbf{Q}$ is $d^2$, and we are done. □

**Claim 2.** *There set* $\bigcap_{j\in\{1,\dots,d\}} A_j$ *consists of a unique point.*

*Proof.* First, some preliminaries. Let $\{\mathbf{r}_1^{\mathrm{T}}, \dots, \mathbf{r}_d^{\mathrm{T}}\}$ denote the rows of the matrix $\mathbf{V}^{-1}$, so that

$$\begin{bmatrix} \mathbf{r}_1^{\mathrm{T}} \\ \vdots \\ \mathbf{r}_d^{\mathrm{T}} \end{bmatrix} \equiv \mathbf{V}^{-1} \tag{43}$$

Since $\mathbf{V}^{-1}$ is invertible, it follows that the vectors $\{\mathbf{r}_1, \dots, \mathbf{r}_d\} \subset \mathbb{R}^d$ are linearly independent. Furthermore, since $\mathbf{V}^{-1}\mathbf{V} = \mathbf{I}$, it follows that $\mathbf{r}_j^{\mathrm{T}}\mathbf{V} = \mathbf{e}_j^{\mathrm{T}}$ for all $j \in \{1, \dots, d\}$. Finally, for all $j \in \{1, \dots, d\}$, and for all $\mathbf{x}^{(1)}, \mathbf{x}^{(2)} \in A_j$, it follows that the difference $\mathbf{x}^{(1)} - \mathbf{x}^{(2)}$ is orthogonal to $\mathbf{r}_j$. To see this consider

$$\begin{aligned} \mathbf{r}_j^{\mathrm{T}}(\mathbf{x}^{(1)} - \mathbf{x}^{(2)}) &= \mathbf{r}_j^{\mathrm{T}}\left(\left(\mathbf{V}(\boldsymbol{\Lambda}-\lambda_j\mathbf{I})\mathbf{V}^{-1}\mathbf{z}^{(1)} + e^{\lambda_j T}\boldsymbol{\mu}_L(0)\right) - \left(\mathbf{V}(\boldsymbol{\Lambda}-\lambda_j\mathbf{I})\mathbf{V}^{-1}\mathbf{z}^{(2)} + e^{\lambda_j T}\boldsymbol{\mu}_L(0)\right)\right) \\ &= \mathbf{r}_j^{\mathrm{T}}\mathbf{V}(\boldsymbol{\Lambda}-\lambda_j\mathbf{I})\mathbf{V}^{-1}(\mathbf{z}^{(1)} - \mathbf{z}^{(2)}) \\ &= \mathbf{e}_j^{\mathrm{T}}(\boldsymbol{\Lambda}-\lambda_j\mathbf{I})\mathbf{V}^{-1}(\mathbf{z}^{(1)} - \mathbf{z}^{(2)}) \\ &= \mathbf{0}^{\mathrm{T}}\mathbf{V}^{-1}(\mathbf{z}^{(1)} - \mathbf{z}^{(2)}) \\ &= 0 \end{aligned} \tag{44}$$

Now, we have already established that $\bigcap_{j\in\{1,\dots,d\}} A_j$ contains at least one point $\mathbf{x}$. Suppose there was some $\mathbf{x}' \in \mathbb{R}^d$ such that $\mathbf{x}' \neq \mathbf{x}$ which was also in $\bigcap_{j\in\{1,\dots,d\}} A_j$. From Equation (44), it follows that $\mathbf{x}-\mathbf{x}'$ is orthogonal to all $\mathbf{r}_j$, where $j \in \{1,\dots,d\}$. This can equivalently be written as $\mathbf{V}^{-1}(\mathbf{x}-\mathbf{x}') = \mathbf{0}$. Since $\mathbf{V}^{-1}$ is invertible, this implies that $\mathbf{x}-\mathbf{x}' = \mathbf{0}$ or that $\mathbf{x} = \mathbf{x}'$, which is a contradiction. It follows that our of assumption of the distinct $\mathbf{x}' \in \bigcap_{j\in\{1,\dots,d\}} A_j$ was false and that $\mathbf{x}$ is the unique point in $\bigcap_{j\in\{1,\dots,d\}} A_j$. □

Now, what does all this mean? If we include Equations (35) as constraints in SDP (44), we are restricting the set of feasible $\tilde{\boldsymbol{\mu}}_L(T)$ vectors to at most one point $\tilde{\boldsymbol{\mu}}_L(T)^*$. As long as the other constraints (e.g., the LMIs) do not exclude $\tilde{\boldsymbol{\mu}}_L(T)^*$, it will be the only feasible $\tilde{\boldsymbol{\mu}}_L(T)$ vector for the problem. Since the objective function depends only on $\tilde{\boldsymbol{\mu}}_L(T)$, it then doesn't matter whether we attempt to maximize or minimize the objective function, the optimal value will simply be the objective function evaluated at $\tilde{\boldsymbol{\mu}}_L(T)^*$. This means that the upper and lower bounds that we calculate, in theory, will be the same.

The astute reader might find it odd that, in the analysis above, we have chosen our set $\mathcal{R}$ to match the eigenvalues of the matrix $\mathbf{A}_L$, while in Section III E we identified the smallest-magnitude eigenvalues of the infinitesimal generator matrix $\mathbf{G}$ as being important. This apparent disconnect is resolved by the observation that, in the absence of the closure problem, there is a close connection between the eigenvalues of the matrices $\mathbf{G}$ and those of $\mathbf{A}_L$. We are not able to state this connection with mathematical precision at present. However, we have noticed, for several such problems, that the smallest magnitude eigenvalues of $\mathbf{G}$ are equal to those of $\mathbf{A}_L$.
